# Supplementary material for: Greedy Algorithms make Efficient Mechanisms
Source: arXiv:1503.05608 source file (2015-03-18)
Supplement: Supplementary file 1 [file sec_appendix_dualFitting.tex]

\section{Dual Fitting - Cont.}
\label{app:DualFitting}

We explain the origin of the dual linear program presented in Section \ref{sec:DualFitting}. The linear program we describe here is a relaxed formulation of the scheduling problem, that has been previously used to solve several related offline and online value maximization problems \cite{JMNY11,JMNY12,LMNY13}. The linear program, also known as the primal program, holds a variable $y_j^i(t)$ representing the allocation of a job $j\in\JobInput$ on server $i$ at time $t\in [a_j,d_j]$.
\\

\noindent \textbf{Primal Program.}
    \begin{alignat}{5}
          \max
          \label{eq:PrimalObjective} & \quad \,\,\,\,\,\,
          \sum_{j\in\JobInput} \, \sum_{i=1}^{C} \intop_{a_j}^{d_j} \, \vd_j y_j^i(t)dt & \\
          \label{eq:PrimalDemand} & \quad
          \,\,\,\,\,\,\,\sum_{i=1}^{C} \intop_{a_j}^{d_j} \,  y_j^i(t)dt \,\,\le\,\, D_{j} & \,\,\,\,\, & \quad \forall j \\
          \label{eq:PrimalCapacity} & \quad \sum_{j:t \in [a_j,d_j]} y_j^i(t) \,\,\le\,\, 1 & \,\,\,\,\, & \quad \forall i,t \\
          \label{eq:PrimalGapDecreasing} & \quad
          \,\,\,\,\,\,\,\sum_{i=1}^{C} y_j^i(t) - \frac{1}{D_j} \cdot  \sum_{i=1}^{C} \intop_{a_j}^{d_j} y_j^i(t)dt \,\,\le\,\, 0 & \,\,\,\,\, & \quad \forall j,t\in [a_j,d_j] \\
          & \quad \,\,\,\,\,\,\,\,\,\,y_j^i(t) \ge 0 & \,\,\,\,\, & \quad \forall j,i,t \in [a_j,d_j] \nonumber
    \end{alignat}

\noindent
The first two sets of constraints \eqref{eq:PrimalDemand},\eqref{eq:PrimalCapacity} are standard demand and capacity constraints. The last constraints \eqref{eq:PrimalGapDecreasing} are gap-reducing constraints, first introduced by \cite{JMNY11}.
These constraints limit the strength of the optimal fractional solution. The first expression in \eqref{eq:PrimalGapDecreasing} is the total amount of (fractional) resources allocated to job $j$ at time $t$; the second expression is the completed fraction of job $j$. For example, if a job is $50\%$ completed, every variable $y_j(t)$ is not allowed to exceed $0.5$ in the fractional solution. Note that for the single server case, the gap-reducing constraints \eqref{eq:PrimalGapDecreasing} are redundant, since they are implied by \eqref{eq:PrimalCapacity}.
The primal objective \eqref{eq:PrimalObjective} is to maximize the total (fractional) value.
